# Supplementary material for: Hypersim: A Photorealistic Synthetic Dataset for Holistic Indoor Scene Understanding
Source: arXiv:2011.02523 ancillary file (2021-08-18)
Supplement: Supplementary file 1 [file supplementary_material.pdf]

# Hypersim: A Photorealistic Synthetic Dataset for Holistic Indoor Scene Understanding

## Supplementary Material

Mike Roberts   Jason Ramapuram   Anurag Ranjan   Atulit Kumar  
Miguel Angel Bautista   Nathan Paczan   Russ Webb   Joshua M. Susskind  
Apple

<http://github.com/apple/ml-hypersim>

### 1. Computational Pipeline Details

**Estimating Free Space** For each of our scenes, we compute an occupancy volume of the scene’s free space using the following space carving algorithm. We begin by rasterizing the scene’s triangle mesh into our occupancy volume, where we mark every covered voxel as occupied. Next, we assume that our artist-defined camera positions are in free space, and we shoot rays in a dense set of directions starting from these camera positions. We raycast against our mesh and the current occupancy volume to obtain the length of each ray before it intersects our scene geometry. After obtaining the length of each ray, we mark every interior voxel along each ray as free in our occupancy volume. Next, we use our updated occupancy volume to sample new positions in the free space uniformly at random, and we repeat our space carving algorithm at these new positions. We repeat this algorithm for several iterations to obtain a conservative estimate of the free space that can be reached from our initial set of artist-defined camera poses. We store our occupancy volume efficiently in an OctoMap data structure [4].

**Generating Camera Trajectories** We generate camera trajectories according to the following sampling procedure. Suppose  $\mathbf{c}_0, \mathbf{c}_1, \dots, \mathbf{c}_K$  is the sequence of camera poses we want to generate. We set  $\mathbf{c}_0$  to be an artist-defined camera pose, and we generate subsequent camera poses by repeatedly sampling from the following conditional probability distribution,

$$p(\mathbf{c}_{i+1}|\mathbf{c}_i) \propto v(\mathbf{c}_{i+1}) \text{ subject to } \mathbf{c}_{i+1} \in N(\mathbf{c}_0, \mathbf{c}_i) \quad (1)$$

where  $\mathbf{c}_{i+1}$  is the unknown next camera pose we would like to sample;  $\mathbf{c}_i$  is the known current camera pose;  $v(\mathbf{c}_{i+1})$  is the view saliency of  $\mathbf{c}_{i+1}$ ; and the constraint  $\mathbf{c}_{i+1} \in N(\mathbf{c}_0, \mathbf{c}_i)$  enforces that  $\mathbf{c}_{i+1}$  is in a small local neighborhood around  $\mathbf{c}_i$ , a larger local neighborhood around  $\mathbf{c}_0$ , is upright, and is in free space. During each iteration of this sampling procedure, we generate a discrete

set of candidate poses in  $N(\mathbf{c}_0, \mathbf{c}_i)$  uniformly at random, compute the un-normalized probability of each candidate by raycasting against our scene geometry, and sample our next camera pose from this discrete set of candidates based on their probabilities.

In our implementation, we use a two-body parameterization of camera pose, similar to [8], where each camera pose  $\mathbf{c}_i$  consists of a look-from position  $\mathbf{p}_i$ , a look-at position  $\mathbf{t}_i$ , and a roll angle  $\phi_i$ . Using this notation, we can express the constraint  $\mathbf{c}_{i+1} \in N(\mathbf{c}_0, \mathbf{c}_i)$  more precisely. In order for the camera pose  $\mathbf{c}_{i+1}$  to be in the set  $N(\mathbf{c}_0, \mathbf{c}_i)$ , the following conditions must be satisfied,

- *Upright:*  $\phi_{i+1}$  must be in the range  $[-5, 5]$  degrees.
- *Obstacle-free:*  $\mathbf{p}_{i+1}$  and  $\mathbf{t}_{i+1}$  must be in free space.
- *Visible:*  $\mathbf{p}_{i+1}$  must be visible from  $\mathbf{p}_i$ , and  $\mathbf{t}_{i+1}$  must be visible from  $\mathbf{t}_i$ .
- *Close to the current camera pose:*

$$\begin{aligned} -\mathbf{b}_{\text{current}} &\leq \mathbf{p}_{i+1} - \mathbf{p}_i \leq \mathbf{b}_{\text{current}} \\ -\mathbf{b}_{\text{current}} &\leq \mathbf{t}_{i+1} - \mathbf{t}_i \leq \mathbf{b}_{\text{current}} \end{aligned} \quad (2)$$

- *Close to the initial camera pose:*

$$\begin{aligned} -\mathbf{b}_{\text{initial}} &\leq \mathbf{p}_{i+1} - \mathbf{p}_0 \leq \mathbf{b}_{\text{initial}} \\ -\mathbf{b}_{\text{initial}} &\leq \mathbf{t}_{i+1} - \mathbf{t}_0 \leq \mathbf{b}_{\text{initial}} \end{aligned} \quad (3)$$

where  $\mathbf{b}_{\text{current}} = [1.5, 1.5, 0.25]^T$  specifies the size in meters of a box-shaped region around the current camera pose;  $\mathbf{b}_{\text{initial}} = [\infty, \infty, 0.25]^T$  specifies a similar box-shaped region around the initial camera pose; and the  $z$ -axis points up. We obtain the initial look-at position  $\mathbf{t}_0$  by raycasting against our scene geometry, and we set  $\alpha = 1$  and  $\beta = 2$  in our view saliency model (see equation 1 in the main paper), indicating that our model is quadratically more sensitive to empty pixels than triangle counts.

**Modifying V-Ray Scenes and Post-Processing** After generating camera trajectories, our next step is to add the trajectories to our V-Ray scene description file. We perform

this modification programmatically using the V-Ray Python API. As we are modifying our V-Ray scene, we configure it to output all the ground truth layers we need for our dataset, and we configure various scene parameters to ensure consistent rendering quality. Our procedure for modifying the V-Ray scene guarantees that each rendered image satisfies the following equation,

$$I = AS + R \quad (4)$$

where  $I$  is the final color image;  $A$  is the diffuse reflectance image;  $S$  is the diffuse illumination image;  $R$  is the non-diffuse residual image; and we add and multiply independently per-pixel and per-color-channel.

At this step in our pipeline, we do not yet have a semantically labeled triangle mesh, so V-Ray cannot output *semantic instance images* (Figure 1d in the main paper) or *semantic label images* (Figure 1e in the main paper) directly. Instead, we configure V-Ray to output *object part images*, i.e., images where each object part in the scene has a unique ID. In a final post-processing step, we use the output of our mesh annotation tool to convert these *object part images* into *semantic instance images* and *semantic label images*. This strategy enables us to render images while annotating our scenes in parallel, and also enables us to re-annotate our scenes (e.g., with a different set of labels) without needing to re-render images.

**Cloud Rendering** After modifying our V-Ray scene, our next step is to render it using a cloud rendering system that we built on top of publicly available cloud computing services. In particular, we use a service that offers a pay-per-minute-per-core licensing model for V-Ray, which is well-suited for bursty rendering workloads (e.g., generating our dataset) and lightweight experiments. This service also provides a powerful Python API for manipulating rendering jobs and performing custom work on each compute node. Our cloud rendering system uses this Python API to programmatically submit rendering jobs, perform custom post-processing tasks on each compute node, and collect rendering statistics.

*Output.* We used our cloud rendering system to generate our entire dataset of 77,400 images at  $1024 \times 768$  resolution, and we scaled up to 100 compute nodes rendering images in parallel.

## 2. Experimental Details

**Tone Mapping** The images in our dataset are stored in an unclamped HDR format, but our real-world test images are LDR images in the range  $[0, 1]$ . To account for this domain gap, we apply the following tone-mapping method [6] to our images during training. We scale each image and apply gamma correction, such that the 90th-percentile brightness value in our original image has a new brightness value of

0.8 after scaling and gamma correction. We then clamp our scaled and gamma-corrected image to the range  $[0, 1]$ .

**Semantic Segmentation** We use an identical training recipe during pre-training and fine-tuning. During each training phase, we train for 100 epochs. We use a one-cycle [10] cosine learning rate schedule [7] with an initial learning rate of 0.01 and a linear warm-up of 3 epochs [2]. We use a distributed data-parallel training strategy with an effective batch size of 64 images per batch (8 images per batch per replica  $\times$  8 replicas), and we use cross-replica batch normalization [5] to aggregate batch statistics across replicas.

We apply the following data augmentations during training. We crop<sup>1</sup> each image with a randomly selected scale in the range  $[0.08, 1.0]$ , a randomly selected aspect ratio in the range  $[0.75, 1.33]$ , and we resize our cropped image to a constant final size of  $512 \times 512$ . We also horizontally flip each image with probability 0.5. Finally, we perturb<sup>2</sup> the hue, saturation, and brightness of each image with probability 0.5. When perturbing the hue, saturation, and brightness of our image, we randomly select a *hue factor* in the range  $[-0.375, 0.375]$ , a *saturation factor* in the range  $[0.25, 1.75]$ , and a *brightness factor* in the range  $[0.25, 1.75]$ . When pre-training on our dataset, we apply tone mapping before data augmentation.

**3D Shape Prediction** When training our Mesh-R-CNN model [1], we follow the authors’ training recipe exactly, except we use a *base learning rate* of 0.005 (instead of the recommended value of 0.02) during pre-training.

Our dataset is annotated with NYU40 labels [3, 9], but Pix3D [11] is annotated with a 9-class label set that only partially overlaps with NYU40. To account for this mismatch, we exclude all instances during pre-training except those belonging to the following NYU40 classes: *bed*, *chair*, *sofa*, *table*, *bookshelf* (*bookcase*), *desk*, *dresser* (*wardrobe*), *pillow* (*misc*), *refrigerator* (*misc*), *television* (*misc*), *box* (*misc*), *nightstand* (*table*), *sink* (*misc*). We indicate our mapping from NYU40 to Pix3D classes in parentheses for all ambiguous cases. We found that Mesh-R-CNN training can become numerically unstable when a mesh extends beyond the training image’s camera frustum, so we exclude any such instances during pre-training.

## References

- [1] Georgia Gkioxari, Jitendra Malik, and Justin Johnson. Mesh R-CNN. In *ICCV 2019*. 2
- [2] Priya Goyal, Piotr Dollár, Ross Girshick, Pieter Noordhuis, Lukasz Wesolowski, Aapo Kyrola, Andrew Tulloch, Yangqing Jia, and Kaiming He. Accurate, large minibatch SGD: Training ImageNet in 1 hour. arXiv 2017. 2

<sup>1</sup> <https://pytorch.org/vision/stable/transforms.html#torchvision.transforms.RandomResizedCrop>

<sup>2</sup> <https://pytorch.org/vision/stable/transforms.html#torchvision.transforms.ColorJitter>

- [3] Saurabh Gupta, Pablo Arbelaez, and Jitendra Malik. Perceptual organization and recognition of indoor scenes from RGB-D images. In *CVPR 2013*. 2
- [4] Armin Hornung, Kai M. Wurm, Maren Bennewitz, Cyrill Stachniss, and Wolfram Burgard. OctoMap: An efficient probabilistic 3D mapping framework based on octrees. *Autonomous Robots*, 34(3), 2013. 1
- [5] Sergey Ioffe and Christian Szegedy. Batch normalization: Accelerating deep network training by reducing internal covariate shift. In *ICML 2015*. 2
- [6] Zhengqi Li and Noah Snavely. CGIntrinsics: Better intrinsic image decomposition through physically-based rendering. In *ECCV 2018*. 2
- [7] Ilya Loshchilov and Frank Hutter. SGDR: Stochastic gradient descent with warm restarts. In *ICLR 2017*. 2
- [8] John McCormac, Ankur Handa, Stefan Leutenegger, and Andrew J. Davison. SceneNet RGB-D: Can 5M synthetic images beat generic ImageNet pre-training on indoor segmentation? In *ICCV 2017*. 1
- [9] Nathan Silberman, Pushmeet Kohli, Derek Hoiem, and Rob Fergus. Indoor segmentation and support inference from RGBD images. In *ECCV 2012*. 2
- [10] Leslie N. Smith and Nicholay Topin. Super-convergence: Very fast training of neural networks using large learning rates. *arXiv 2017*. 2
- [11] Xingyuan Sun, Jiajun Wu, Xiuming Zhang, Zhoutong Zhang, Chengkai Zhang, Tianfan Xue, Joshua B. Tenenbaum, and William T. Freeman. Pix3D: Dataset and methods for single-image 3D shape modeling. In *CVPR 2017*. 2
